# Supplementary material for: Stimulated amplification of propagating spin waves
Source: arXiv:2208.11455 ancillary file (2023-11-01)
Supplement: Supplementary file 1 [file Supplement.pdf]

## Supplementary material

-

### Stimulated amplification of propagating spin waves

D. Breitbach,<sup>1</sup> M. Schneider,<sup>1</sup> F. Kohl,<sup>1</sup> L. Scheuer,<sup>1</sup> B. Heinz,<sup>1</sup> R. O. Serha,<sup>1,2</sup> J. Maskill,<sup>1</sup> T. Brächer,<sup>1</sup>  
B. Lägél,<sup>1</sup> C. Dubs,<sup>3</sup> V. S. Tiberkevich,<sup>4</sup> A. N. Slavin,<sup>4</sup> A. A. Serga,<sup>1</sup> B. Hillebrands,<sup>1</sup>  
A. V. Chumak<sup>2</sup> and P. Pirro<sup>1</sup>

<sup>1</sup>*Fachbereich Physik and Landesforschungszentrum OPTIMAS,  
Technische Universität Kaiserslautern, D-67663 Kaiserslautern, Germany*

<sup>2</sup>*Faculty of Physics, University of Vienna, A-1090 Vienna, Austria*

<sup>3</sup>*INNOVENT e.V. Technologieentwicklung, Jena, Germany*

<sup>4</sup>*Department of Physics, Oakland University, Rochester, MI, USA*

#### I. FREQUENCY OF THE AMPLIFIED SPIN-WAVE PACKET

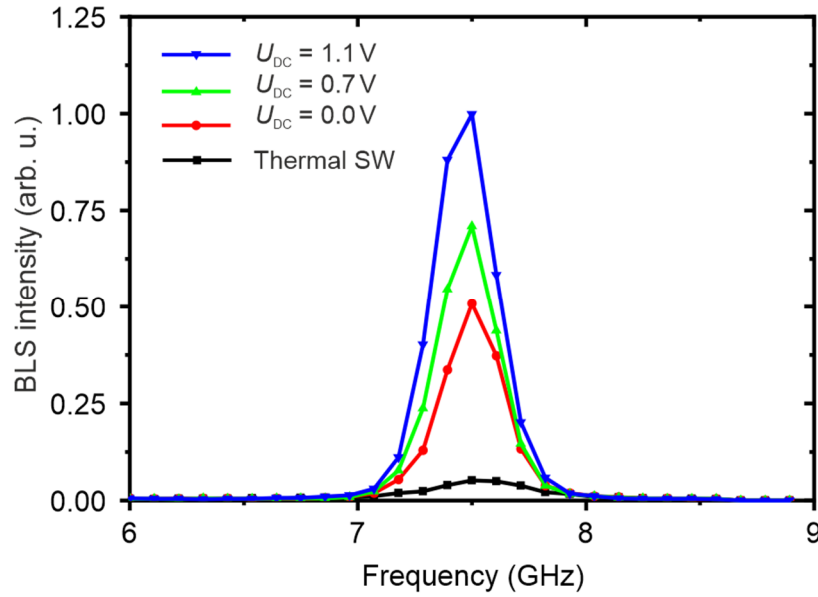

**Supplementary Fig. 1:** BLS frequency of the spin-wave packet for different DC pulse amplitudes/amplification levels. The frequency of the spin-wave packet is preserved in the amplification process. **Black:** Thermal spin-wave spectrum for comparison.

## II. INFLUENCE OF THE RF FREQUENCY ON THE AMPLIFICATION FACTOR

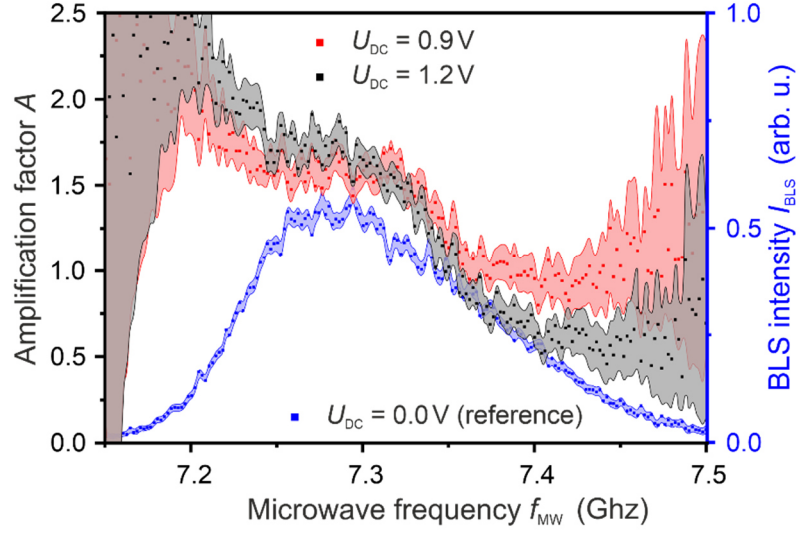

**Supplementary Fig. 2:** **Left scale:** Amplification factor as a function of the microwave frequency used for spin-wave excitation, for two different DC pulse voltages (red, black curves). **Right scale:** BLS intensity of the spin-wave packet as a function of the microwave frequency without DC pulse ( $U_{DC} = 0.0\text{ V}$ ) as reference (blue curve).

## III. SPIN-WAVE DISPERSION RELATION AND GROUP VELOCITY

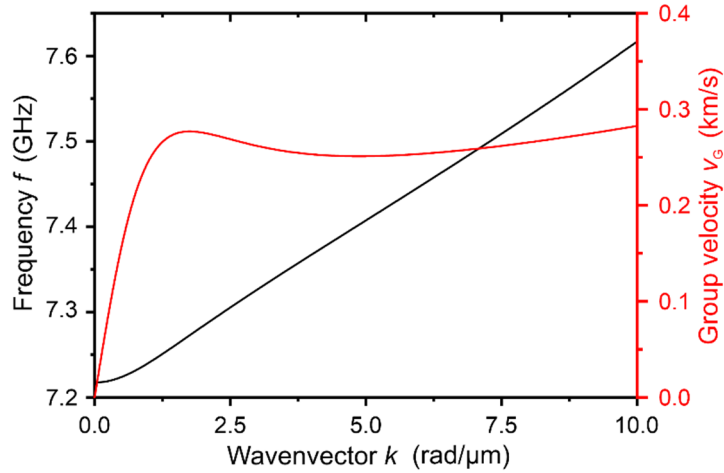

**Supplementary Fig. 3:** **Left scale:** Calculated spin-wave dispersion relation for the fundamental waveguide mode. **Right scale:** Corresponding spin-wave group velocity as a function of the wavevector. Calculations were performed following [S1] and assuming  $M_S = 142.3\text{ kA/m}$ ,  $A = 3.5\text{ pJ/m}$ ,  $t_{YIG} = 34\text{ nm}$ ,  $w_{\text{eff}} = 1.9\text{ }\mu\text{m}$  and  $\mu_0 H_{\text{app}} = 188\text{ mT}$ , additionally taking into account  $\mu_0 H_{\text{demag}} = 3.58\text{ mT}$ .

## References

- S1. B. A. Kalinikos, A. N. Slavin, Theory of dipole-exchange spin wave spectrum for ferromagnetic films with mixed exchange boundary conditions, *Journal of Physics C: Solid State Physics* **19**, 7013 (1986)
